# Supplementary material for: Magnetic Trampoline Resonators from (La,Sr)MnO3 Single-Crystal Thin Films
Source: arXiv:2501.12177 source file (2025-01-21)
Supplement: Supplementary file 1 [file LSMO_trampolines-supplementary.pdf]

*Supplementary Material*

# Magnetic Trampoline Resonators from (La,Sr)$MnO_3$ Single-Crystal Thin Films

Nicola Manca,[1,*] Dhavalkumar Mungpara,[2]
Leonélio Cichetto Jr,[1] Alejandro E. Plaza,[1] Gianrico Lamura,[1]
Alexander Schwarz,[2] Daniele Marré,[3,1] and Luca Pellegrino[1]

[1]*CNR-SPIN, C.so F. M. Perrone, 24, 16152 Genova, Italy*

[2]*Institute of Nanostructure and Solid State Physics, University of Hamburg, Germany*

[3]*Dipartimento di Fisica, Università degli Studi di Genova, 16146 Genova, Italy*

This supplemental material contains the following:

- Section I: Magnetization loops of LSMO(110)
- Section II: Comparison of Resistance vs Temperature in LSMO(110) films

* nicola.manca@spin.cnr.it

## Sec. I. MAGNETIZATION LOOPS OF LSMO(110)

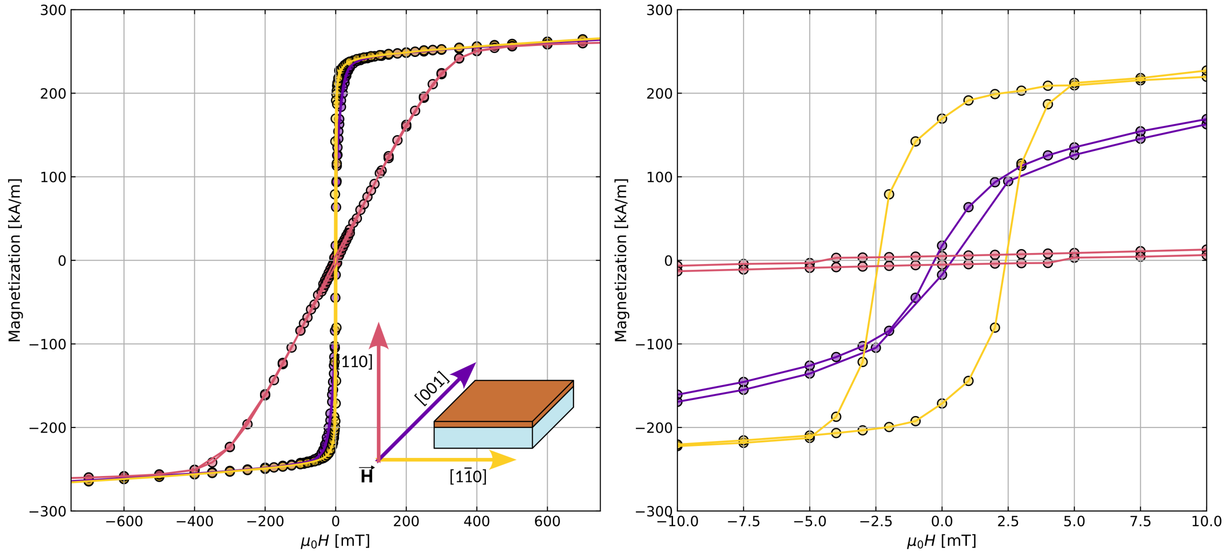


Figure S1. Room-temperature magnetization loops of a bare (La,Sr)$MnO_3$ film measured along the three main lattice directions, as show in the inset of the left panel. The right panel shows the same data but in a narrower range for better comparison.

## Sec. II.    COMPARISON OF RESISTANCE VS TEMPERATURE IN LSMO(110) FILMS

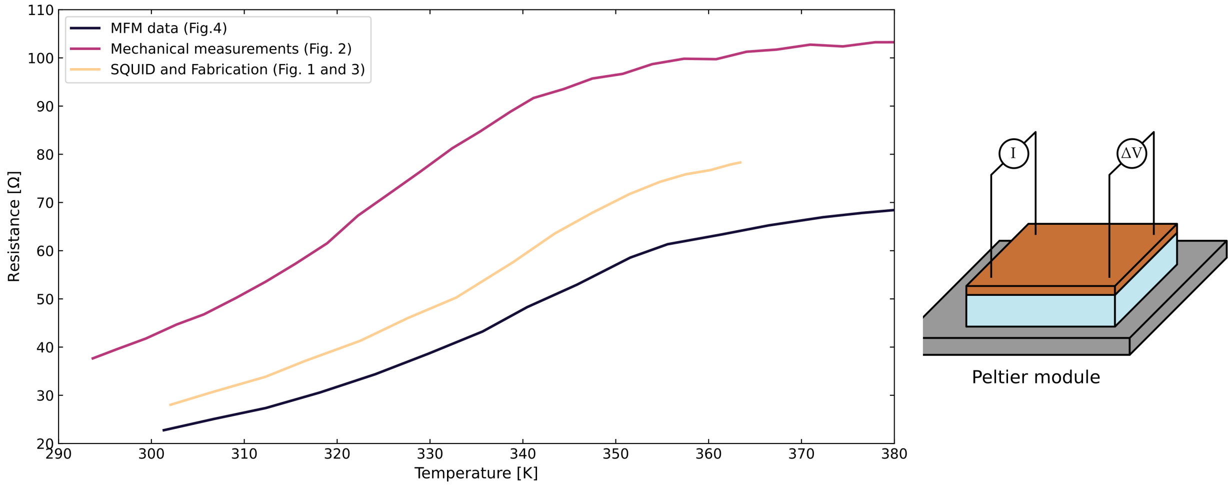


Figure S2.    Resistance vs temperature characteristics of the LSMO thin films employed in this work. Plot labels indicate the use for each sample. The resistance measurements were performed in four-probes configuration with the sample in contact to a Peltier module to control the temperature.
